# Supplementary material for: Quantifying chirality of phonons
Source: arXiv:2604.10231 source file (2026-12-01)
Supplement: Supplementary file 1 [file supp_260411-2.tex]

%===========================
% Supplemental Materials for
% True Chirality of Phonons in Chiral Materials
%===========================
%\documentclass[12pt,a4paper]{report}
\documentclass[aps,prb,superscriptaddress]{revtex4-2}
\usepackage{amsmath,amssymb,graphicx,bm,color,booktabs,multirow}
\usepackage{tabularray}
\usepackage{csquotes}
\usepackage[version=4]{mhchem}
\usepackage{tcolorbox}
\usepackage{rotating}
\usepackage[colorlinks=true,allcolors=blue]{hyperref}
\usepackage{float} 
\makeatletter
% --- minimal fix for revtex4-2 v4.2f "Extra \or" bug, avoids recursion ---
\def\@classz@{\let\@tabclassz\@tabclassiv}
\expandafter\let\csname @xfloat@ORIG\endcsname\@xfloat
\def\@xfloat#1[#2]{%
	\csname @xfloat@ORIG\endcsname#1[#2]%
}
\makeatother

\begin{document}
	
	\title{Supplemental Material:\\Quantifying chirality of phonons}
	
	\author{Yu-Chi Huang}
	\affiliation{Department of Physics, Institute of Science Tokyo, Tokyo 152-8551, Japan}
	\affiliation{Department of Applied Physics and Science Education, Eindhoven University of Technology, Eindhoven 5612 AP, Netherlands.}
	
	\author{Gakuto Kusuno}
	\affiliation{Department of Physics, Institute of Science Tokyo, Tokyo 152-8551, Japan}

	\author{Yusuke Hashimoto}
	\affiliation{Frontier Research Institute for Interdisciplinary Sciences, Tohoku University, Sendai 980-8578, Japan}	
		
	\author{Dominik M. Juraschek}
	\affiliation{Department of Applied Physics and Science Education, Eindhoven University of Technology, Eindhoven 5612 AP, Netherlands.}
	
	\author{Hiroaki Kusunose}
	\affiliation{Department of Physics, Meiji University, Kawasaki 214-8571, Japan}
	
	\author{Takuya Satoh}
	\affiliation{Department of Physics, Institute of Science Tokyo, Tokyo 152-8551, Japan}
	\affiliation{Quantum Research Center for Chirality, Institute for Molecular Science, Okazaki 444-8585, Japan}
	
	\date{\today}
	
	\maketitle
	
	%===========================
	\section{Computational Parameters}
	%===========================
	
	Table~\ref{tab:params} summarizes the computational parameters for the eight materials discussed in the main text.
	Phonon properties were computed using density functional perturbation theory (DFPT)~\cite{Baroni2001} as implemented in the \textsc{abinit}~code~\cite{ABINIT_8.10.3}.
	The plane-wave cutoff energies, $k$-point meshes, exchange-correlation functionals~\cite{Perdew1996}, and pseudopotentials were chosen to ensure 	convergence of both total energies and phonon frequencies.
	GGA-PBE denotes the Perdew--Burke--Ernzerhof generalized gradient approximation, while LDA refers to the local density approximation.
	
    \renewcommand{\thefigure}{S\arabic{figure}}
    \setcounter{figure}{0}
    \renewcommand{\theequation}{S\arabic{equation}}
    \setcounter{figure}{0}
	\renewcommand{\thetable}{S\arabic{table}}
    \setcounter{table}{0}
	\begin{table*}[h]
		\centering
		\caption{Summary of computational parameters for all investigated materials.}
		\begin{tabular}{lcccc}
			\toprule
			Material & Space group & $E_{\text{cut}}$ (Ha) & $k$-mesh & Exchange-Correlation
			Functional \\
			\midrule
			(Chiral) & & & & \\
			$\alpha$-SiO$_2$ (L/R) & $\text{P}3_{2}21/\text{P}3_{1}21$ & 15 & $6\times6\times6$ & GGA-PBE \\
			Se (L/R) & $\text{P}3_{2}21/\text{P}3_{1}21$ & 15 & $8\times8\times6$ & GGA-PBE \\
			Te (L/R) & $\text{P}3_{2}21/\text{P}3_{1}21$ & 15 & $8\times8\times6$ & GGA-PBE \\
			$\alpha$-HgS (L/R) & $\text{P}3_{2}21/\text{P}3_{1}21$ & 60 & $6\times6\times4$ & GGA-PBE \\
			\midrule
			(Achiral) & & & & \\
			Si & $\text{Fd}\bar{3}\textit{m}$ & 15 & $4\times4\times4$ & LDA \\
			GaAs & $\text{F}\bar{4}3\textit{m}$ & 15 & $4\times4\times4$ & GGA-PBE \\
			GaP & $\text{F}\bar{4}3\textit{m}$ & 15 & $4\times4\times4$ & GGA-PBE \\
			ZnTe & $\text{F}\bar{4}3\textit{m}$ & 15 & $4\times4\times4$ & GGA-PBE \\
			\bottomrule
		\end{tabular}
		\label{tab:params}
	\end{table*}
    
%	\newpage
	%===========================
	\section{Momentum-Resolved Dynamical Chirality}
	%===========================
	The momentum-resolved dynamical chirality $\mathbf{L}_j(\mathbf{k})\cdot \hat{\mathbf{k}}$ is computed for all materials. In chiral systems (e.g. Se, Te, and $\alpha$-HgS), the nonzero momentum-resolved dynamical chirality shows opposite signs in left- and right-handed systems in Fig.~S1--3. In noncentrosymmetric achiral systems (e.g. GaP, ZnTe), nonzero momentum-resolved dynamical chirality arises from broken inversion symmetry. Figures S4 and S5 display momentum-resolved dynamical chirality mapping along high-symmetry paths.

	\newpage

	\textbf{Chiral Materials}
	%Se
	\begin{figure*}[h]
		\centering
		\makebox[\textwidth][c]{ % Centers the figure horizontally
			\includegraphics[width=0.76\textwidth]{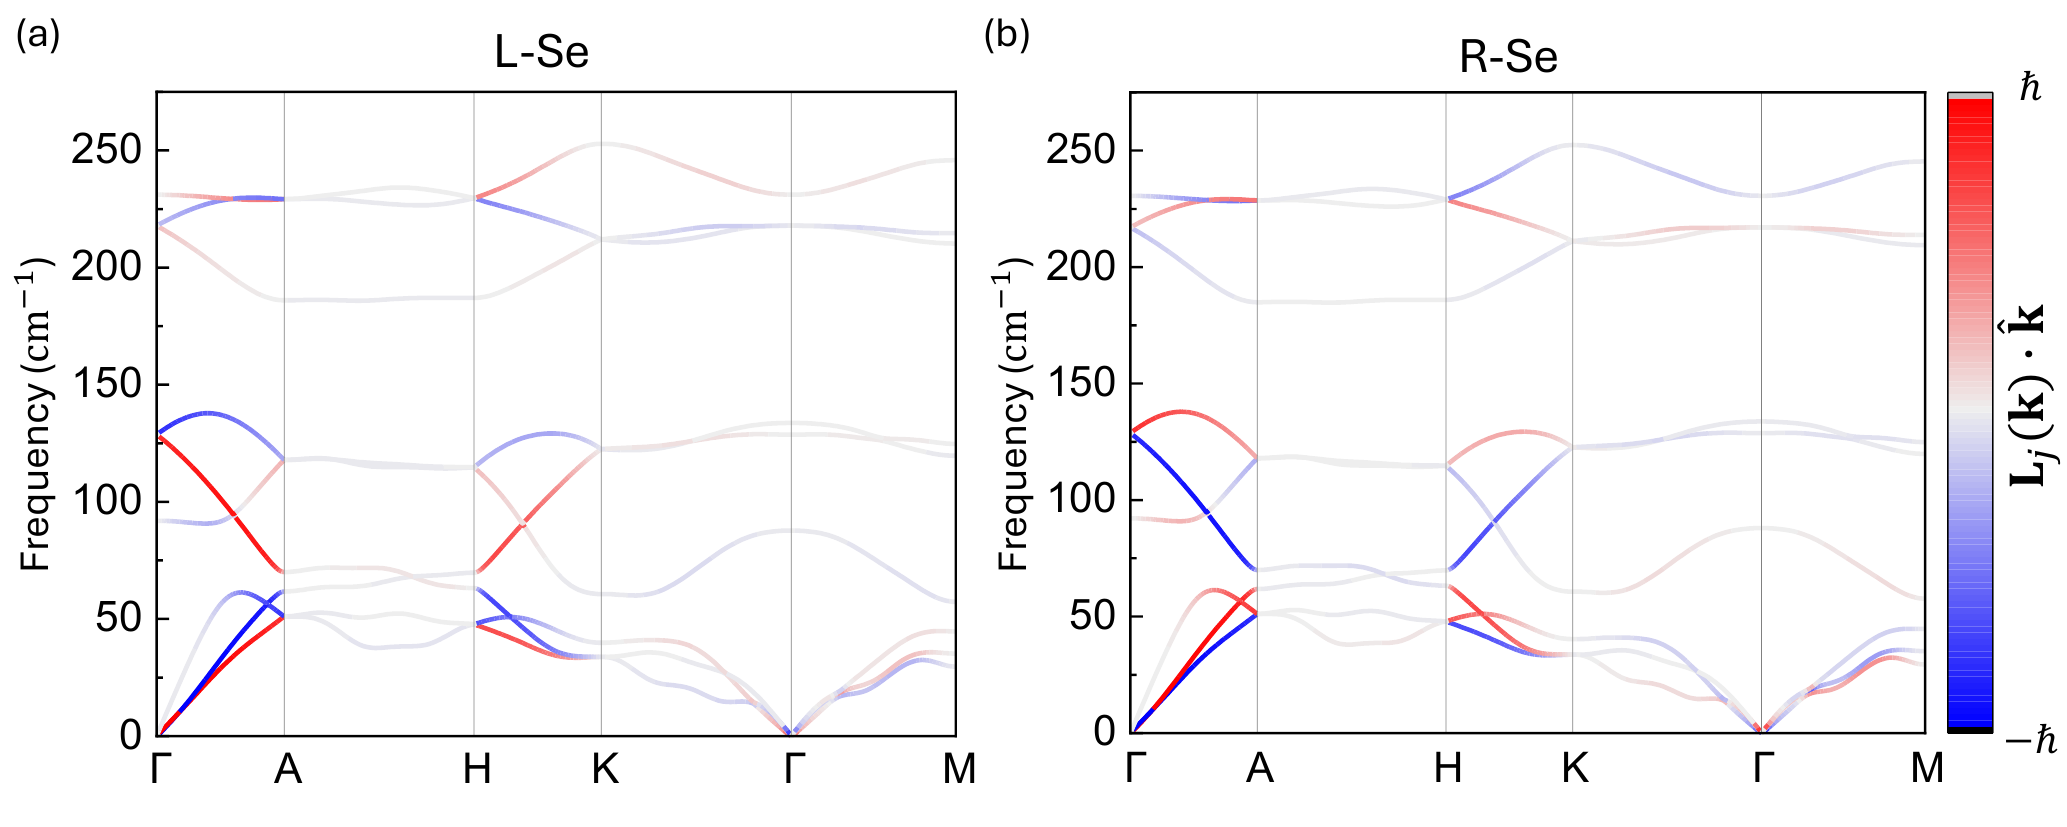}	
		}
		\caption{Momentum-resolved dynamical chirality in (a) L-Se and (b) R-Se along the paths between high symmetry points.}
	\end{figure*}
%	
	%Te
	\begin{figure*}[h]
		\centering
		\makebox[\textwidth][c]{ % Centers the figure horizontally
			\includegraphics[width=0.76\textwidth]{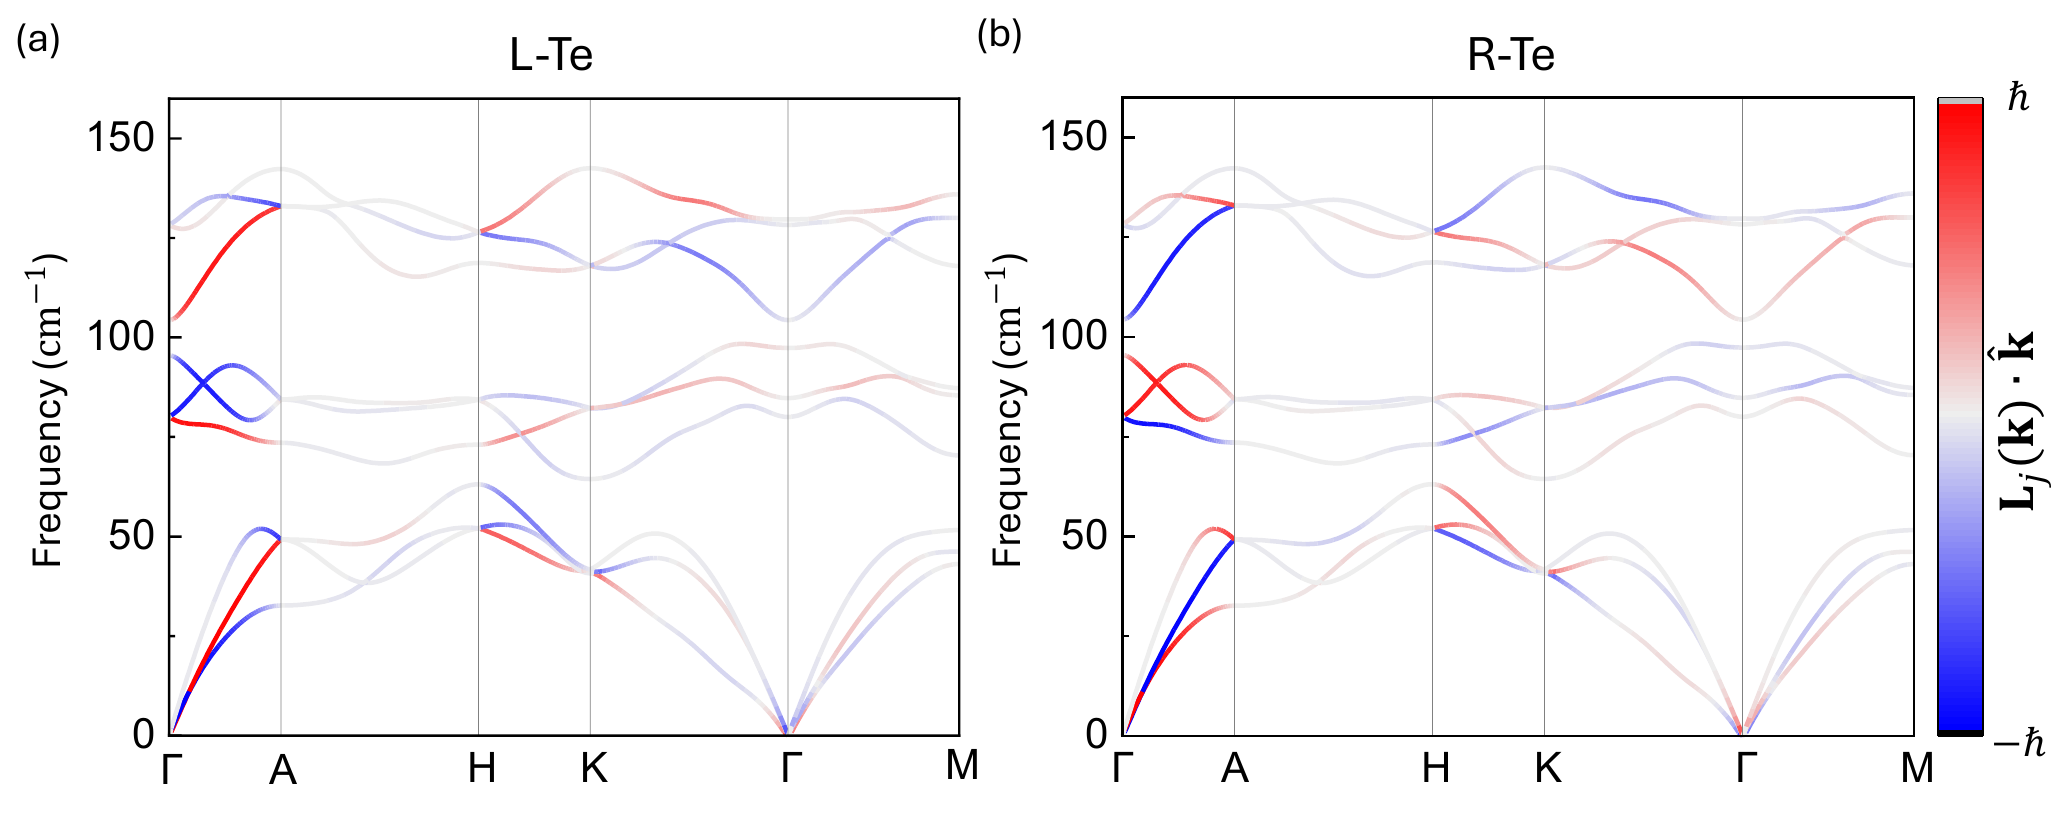}	
		}
		\caption{Momentum-resolved dynamical chirality in (a) L-Te and (b) R-Te along the paths between high symmetry points.}
	\end{figure*}
%	
	%HgS
	\begin{figure*}[h]
		\centering
		\makebox[\textwidth][c]{ % Centers the figure horizontally
			\includegraphics[width=0.76\textwidth]{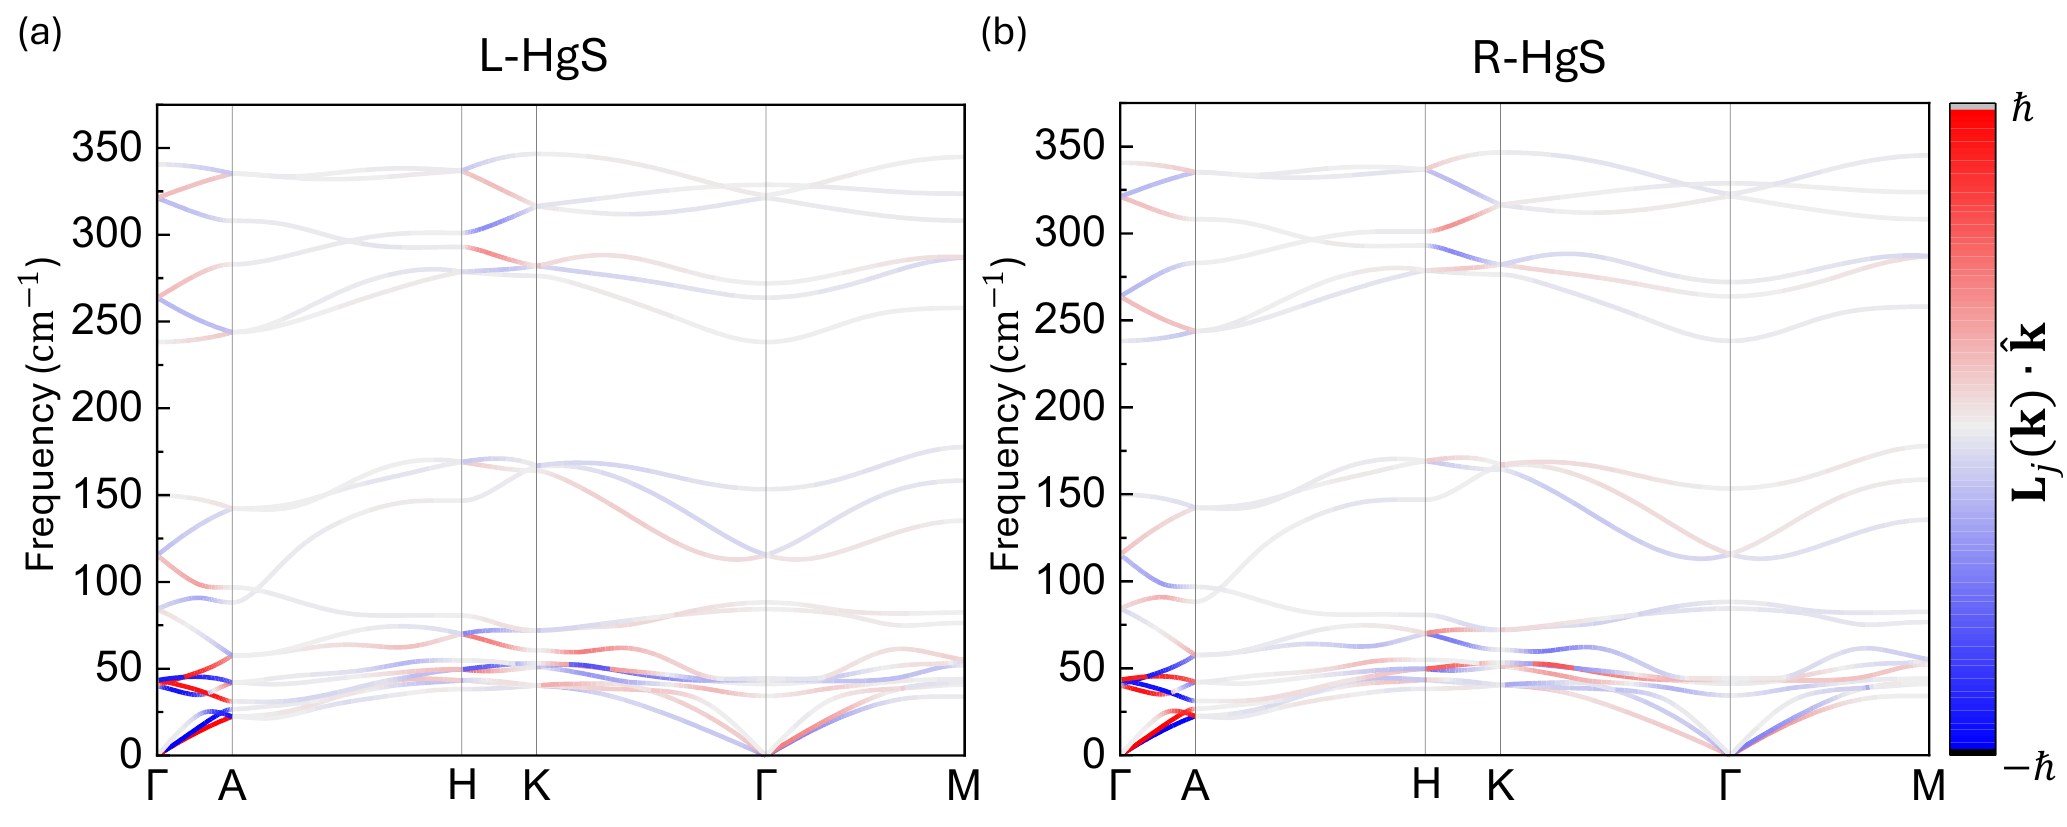}	
		}
		\caption{Momentum-resolved dynamical chirality in (a) L-HgS and (b) R-HgS along the paths between high symmetry points.}
	\end{figure*}
	\clearpage
	
	\textbf{Achiral Materials}
	
	%GaP
	\begin{figure*}[h]
		\centering
		\makebox[\textwidth][c]{ % Centers the figure horizontally
			\includegraphics[width=0.5\textwidth]{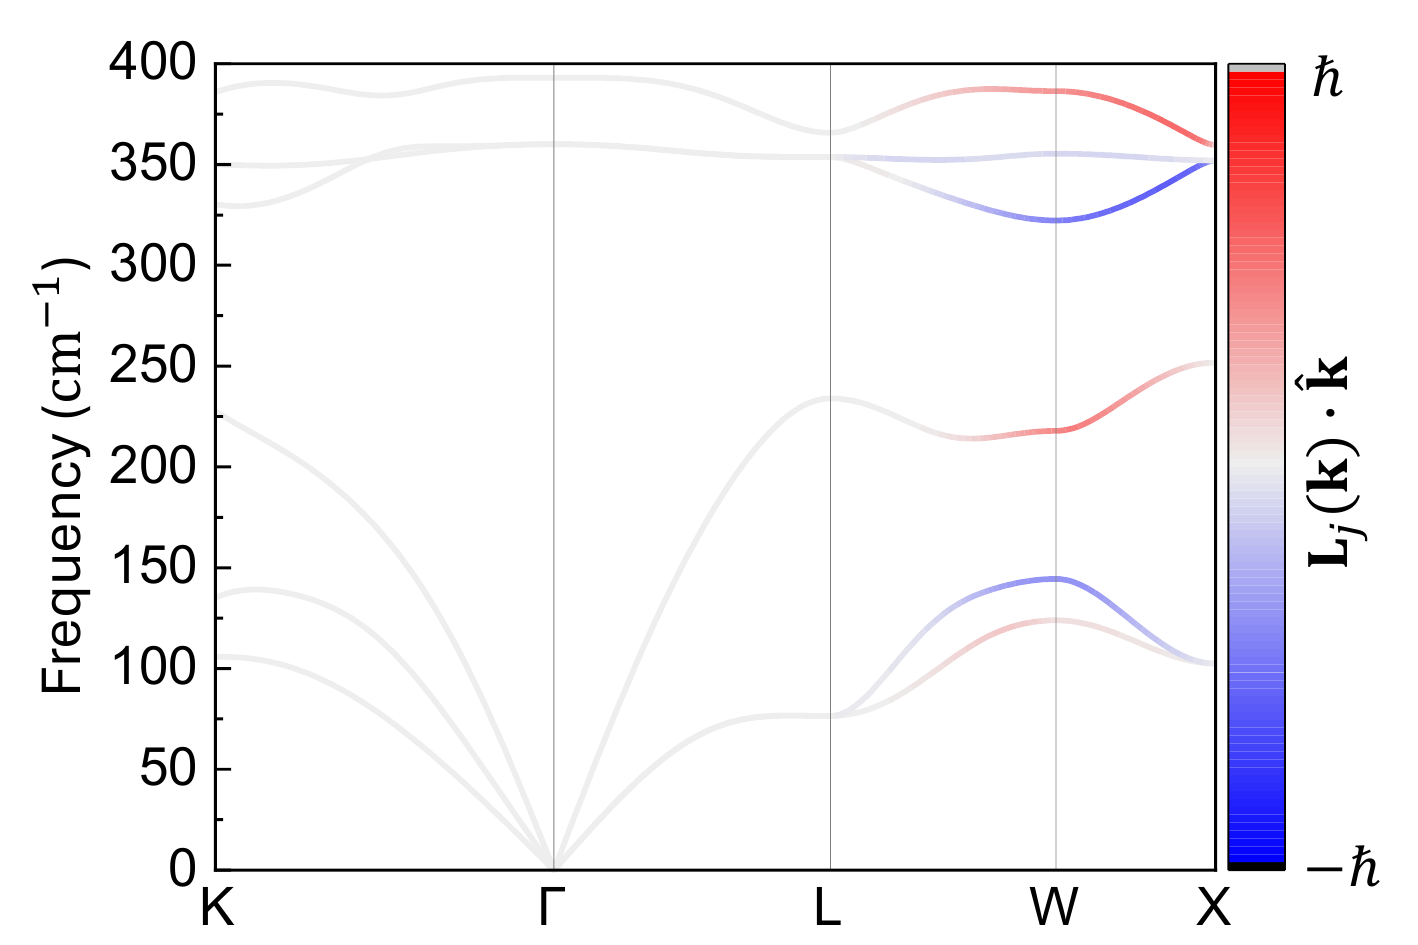}	
		}
		\caption{Momentum-resolved dynamical chirality in GaP along the paths between high symmetry points.}
	\end{figure*}
	%\clearpage
	
	%ZnTe
	\begin{figure*}[h]
		\centering
		\makebox[\textwidth][c]{ % Centers the figure horizontally
			\includegraphics[width=0.5\textwidth]{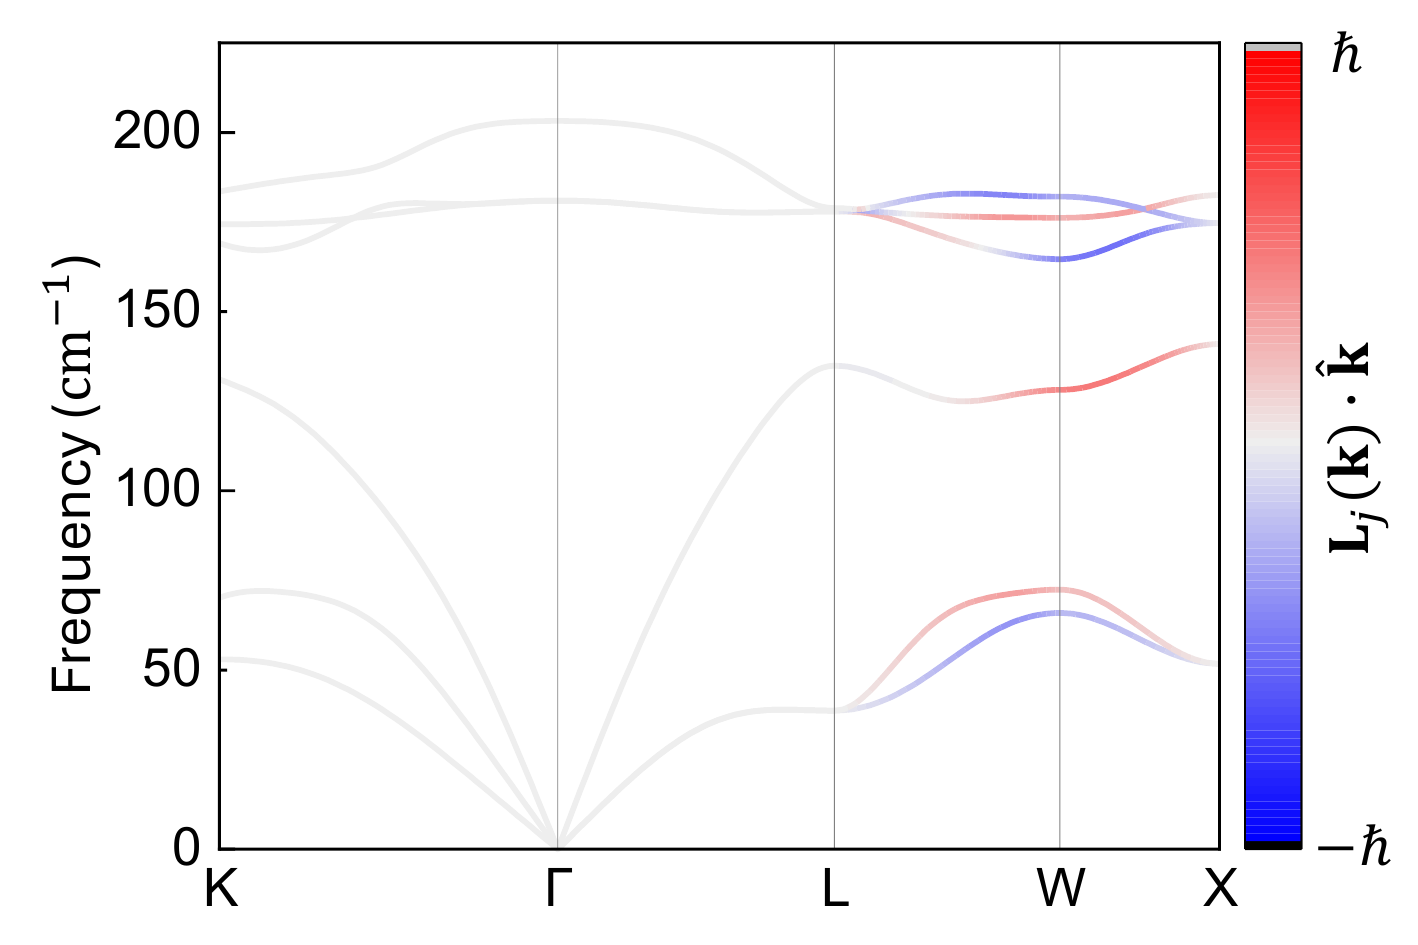}	
		}
		\caption{Momentum-resolved dynamical chirality in ZnTe along the paths between high symmetry points.}
	\end{figure*}
	\clearpage

    \newpage
    \section{Temperature dependence of bulk dynamical chirality as characterized by $G_0$ and $G_u$}
    As shown in Fig.~S6, both $G_0$ and $G_u$ increase approximately proportionally with temperature for all materials. This behavior can be understood from the definitions of $G_0$ and $G_u$,

    {\footnotesize
    \begin{equation}
    \begin{aligned}
    G_0(T) &= \frac{1}{N_0 \hbar}\sum_{j} \sum_{\mathbf{k}}
    f(\omega_j(\mathbf{k}))
    \left[\mathbf{L}_j(\mathbf{k}) \cdot \mathbf{F}_1(\mathbf{k}) \right], \\[0em]
    G_u(T) &= \frac{1}{N_0 \hbar}\sum_{j} \sum_{\mathbf{k}}
    f(\omega_j(\mathbf{k}))
    \frac{1}{2}\left[3L^z_j(\mathbf{k}) F^z_1(\mathbf{k})
    - \mathbf{L}_j(\mathbf{k}) \cdot \mathbf{F}_1(\mathbf{k})\right],
    \end{aligned}
    \end{equation}
    }together with the Bose--Einstein distribution,
    \begin{equation}
    f(\omega_j(\mathbf{k})) = \frac{1}{e^{\hbar \omega_j(\mathbf{k}) / k_B T} - 1}.
    \end{equation}
     In the high-temperature limit ($k_BT \gg \hbar \omega_j(\mathbf{k})$), the distribution can be approximated as $f(\omega_j(\mathbf{k})) \approx \frac{k_BT}{\hbar \omega_j(\mathbf{k})} \propto T$. Accordingly, at sufficiently high temperatures, $G_0$ and $G_u$ can be approximated as
    {\footnotesize
    \begin{equation}
    \begin{aligned}
    G_0(T) &\approx \frac{k_BT}{N_0 \hbar^2}\sum_{j} \sum_{\mathbf{k}}
    \frac{1}{\omega_j(\mathbf{k})}
    \left[\mathbf{L}_j(\mathbf{k}) \cdot \mathbf{F}_1(\mathbf{k}) \right] \propto T, \\[0em]
    G_u(T) &\approx \frac{k_BT}{N_0 \hbar^2}\sum_{j} \sum_{\mathbf{k}}
    \frac{1}{\omega_j(\mathbf{k})}
    \frac{1}{2}\left[3L^z_j(\mathbf{k}) F^z_1(\mathbf{k})
    - \mathbf{L}_j(\mathbf{k}) \cdot \mathbf{F}_1(\mathbf{k})\right] \propto T.
    \end{aligned}
    \end{equation}
    }
    
\clearpage
\refstepcounter{figure}
\label{fig:linear_T_G}
\begin{center}
	\includegraphics[width=0.75\textwidth]{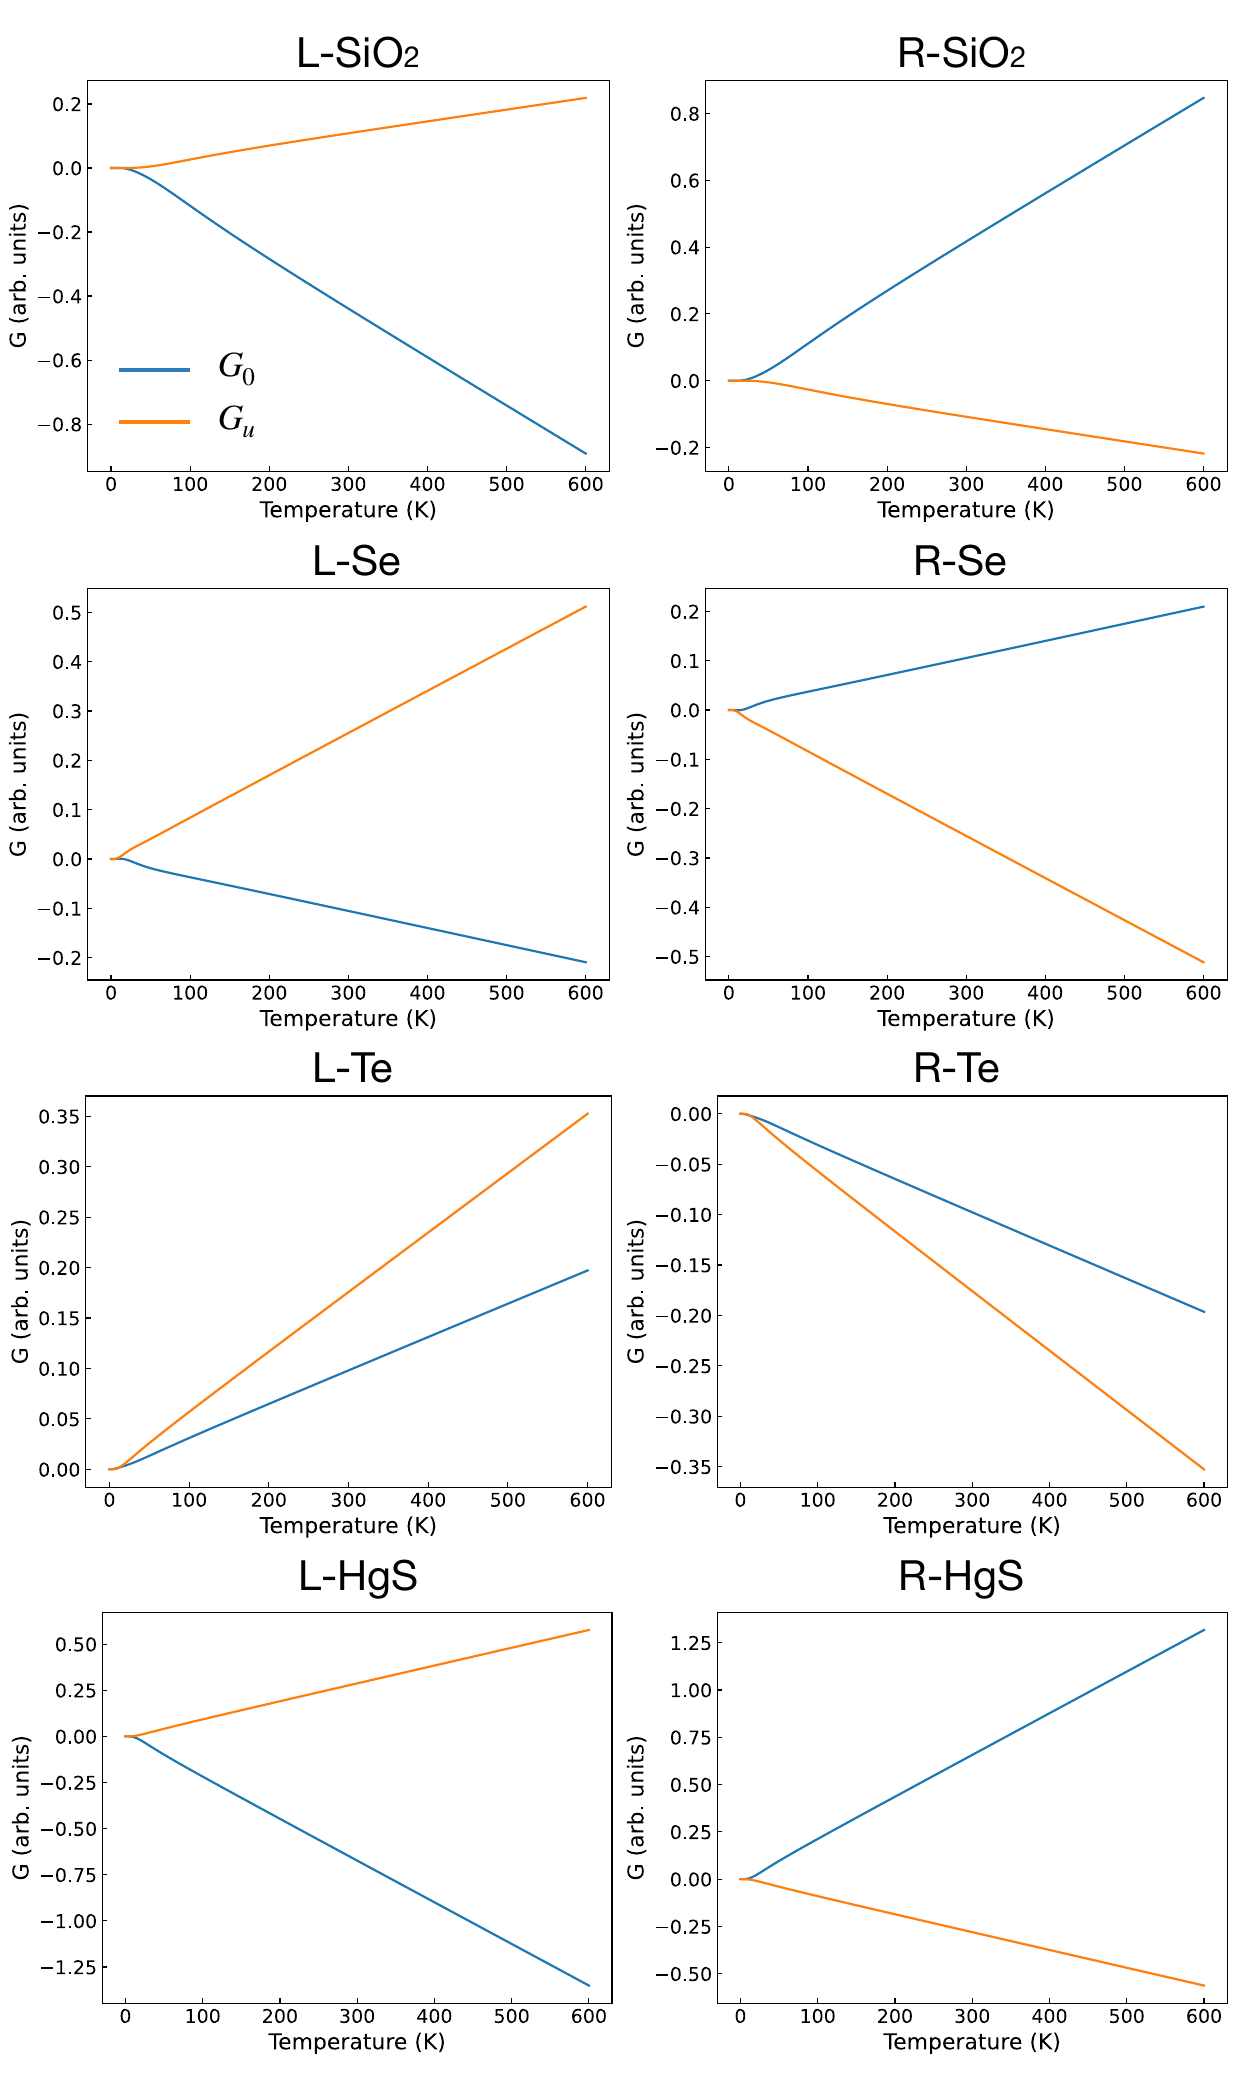}

	\textbf{FIG. \thefigure.} Temperature dependence of bulk dynamical chirality as characterized by $G_0$ and $G_u$.
\end{center}
    
\if0
    \begin{figure}[ht]
		\makebox[\textwidth][c]{ % Centers the figure horizontally
			\includegraphics[width=0.75\textwidth]{figures_supp/linear_T_G.pdf} % Adjust width as needed
		}
		\caption{Temperature dependence of bulk dynamical chirality as characterized by $G_0$ and $G_u$}
	\end{figure}
\fi

	\newpage

	%===========================
	\section{Derivation of Structure Factor $F_1(\mathbf{k})$}
	%===========================
	The structure factors for point groups $D_3$, $O_h$, and $T_d$ are summarized below.
	
	\noindent For $D_3$, the components of $\mathbf{F}_1(\mathbf{k})$ are given by
	{\footnotesize
    \begin{equation}
    \begin{aligned}
    F_1^x(\mathbf{k}) &= \frac{2}{\sqrt{3}}
    \left[ 2 \cos \left(\frac{k_x a}{2}\right)
    + \cos \left(\frac{\sqrt{3} k_y a}{2}\right) \right]
    \sin \left(\frac{k_x a}{2}\right), \\[0.8em]
    F_1^y(\mathbf{k}) &= 2 \cos \left(\frac{k_x a}{2}\right)
    \sin \left(\frac{\sqrt{3} k_y a}{2}\right), \\[0em]
    F_1^z(\mathbf{k}) &= \sin \left(k_z c\right) .
    \end{aligned}
    \end{equation}
    }
	while for $O_h$ and $T_d$, they take the form
	{\footnotesize
    \begin{align}
    \mathbf{F}_1 (\mathbf{k}) = \left(\sin(k_x a),\sin(k_y a),\sin(k_z a)\right).
    \end{align}
    }
	
	\noindent These structure factors can be derived using the projection method in group theory. As an example, we consider the point group $D_3$. First, the $\mathbf{k}$-dependent angular momentum $\mathbf{L}_j(\mathbf{k})$ can be expanded in a Fourier series as
	\begin{align}
		\mathbf{L}_j(\mathbf{k})=c_1(j)\mathbf{F}_1(\mathbf{k})+c_2(j)\mathbf{F}_2(\mathbf{k})+...,
	\end{align}
	where $\mathbf{F}_i(\mathbf{k})$ represent basis functions with different periodicities and $\mathbf{F}_1(\mathbf{k})$ corresponds to the lowest-order term. Next, by applying the projection operator from group theory, we obtain
	\begin{align}
		\mathcal{P}_{\alpha\beta}[\mathbf{L}_j(\mathbf{k})] = c_{\beta} F_1^{\alpha}(\mathbf{k}) \propto F_1^{\alpha}(\mathbf{k}),
	\end{align}
	where $\alpha, \beta = x, y, z$ denote Cartesian components. The projection operator is defined as:
	\begin{align}
		\mathcal{P}_{\alpha\beta} \equiv \frac{d}{g} \sum_{\mathcal{G}} D^*_{\alpha\beta}(\mathcal{G}) \mathcal{G}, 
	\end{align}
	where $d$ is the dimension of irreducible representation, $g$ is the number of symmetry operations, $\mathcal{G}$ is the symmetry operation, and $D_{\alpha\beta}(\mathcal{G})$ is the  representation matrix of $\mathcal{G}$. Hence, we can obtain the relation between the first-order structure function and the projection operation:
	\begin{align}
		F_1^{\alpha}(\mathbf{k}) \propto \mathcal{P}_{\alpha\beta}[\mathbf{L}_j(\mathbf{k})] \propto  \sum_{\mathcal{G}} D^*_{\alpha\beta}(\mathcal{G}) \mathcal{G}[\mathbf{L}_j(\mathbf{k})].
	\end{align}
	
	\noindent In this study, we focus on chiral materials belonging to the point group $D_3$. 
    To construct the structure factor relevant for the evaluation of $G_0$ and $G_u$, we refer to the character table of $D_3$ (Table~S2). 
    The corresponding unit cell vectors are shown in Fig.~S7.
	\begin{table}[h]
		\centering
		\renewcommand{\arraystretch}{2}
		\begin{tabular}{c c c c c c c}
			\toprule
			irrep. & $1$ & $C_2$ & $C_2$ & $C_2$ & $C_3$ & $C_3^{-1}$ \\
			\midrule
			$A_1$ & 1 & 1 & 1 & 1 & 1 & 1 \\
			$A_2$ & 1 & $-1$ & $-1$ & $-1$ & 1 & 1 \\
			\midrule
			$E$ & 
			$\begin{pmatrix} 1 & 0 \\ 0 & 1 \end{pmatrix}$ & 
			$\begin{pmatrix} 1 & 0 \\ 0 & -1 \end{pmatrix}$ & 
			$\begin{pmatrix} -\frac{1}{2} & -\frac{\sqrt{3}}{2} \\ -\frac{\sqrt{3}}{2} & \frac{1}{2} \end{pmatrix}$ & 
			$\begin{pmatrix} -\frac{1}{2} & \frac{\sqrt{3}}{2} \\ \frac{\sqrt{3}}{2} & \frac{1}{2} \end{pmatrix}$ & 
			$\begin{pmatrix} -\frac{1}{2} & -\frac{\sqrt{3}}{2} \\ -\frac{\sqrt{3}}{2} & -\frac{1}{2} \end{pmatrix}$ & 
			$\begin{pmatrix} -\frac{1}{2} & \frac{\sqrt{3}}{2} \\ \frac{\sqrt{3}}{2} & -\frac{1}{2} \end{pmatrix}$ \\
			\midrule
			$\chi_E$ & 2 & 0 & 0 & 0 & $-1$ & $-1$ \\
			\bottomrule
			\toprule
			$\mathcal{G}[\mathbf{a}_x]$ & $\mathbf{a}_x$ & $\mathbf{a}_x$ & $\mathbf{a}_-$ & $\mathbf{a}_+$ & $\mathbf{a}_+$ & $\mathbf{a}_-$ \\
			$\mathcal{G}[\mathbf{a}_z]$ & $\mathbf{a}_z$ & $-\mathbf{a}_z$ & $-\mathbf{a}_z$ & $-\mathbf{a}_z$ & $\mathbf{a}_z$ & $\mathbf{a}_z$ \\
			\bottomrule
		\end{tabular}
		\caption{Table of irreducible representations of $D_3$ and the symmetry operations on unit cell vectors in the materials of $D_3$.}
	\end{table}

	\begin{figure}[h]
		\makebox[\textwidth][c]{ % Centers the figure horizontally
			\includegraphics[width=0.6\textwidth]{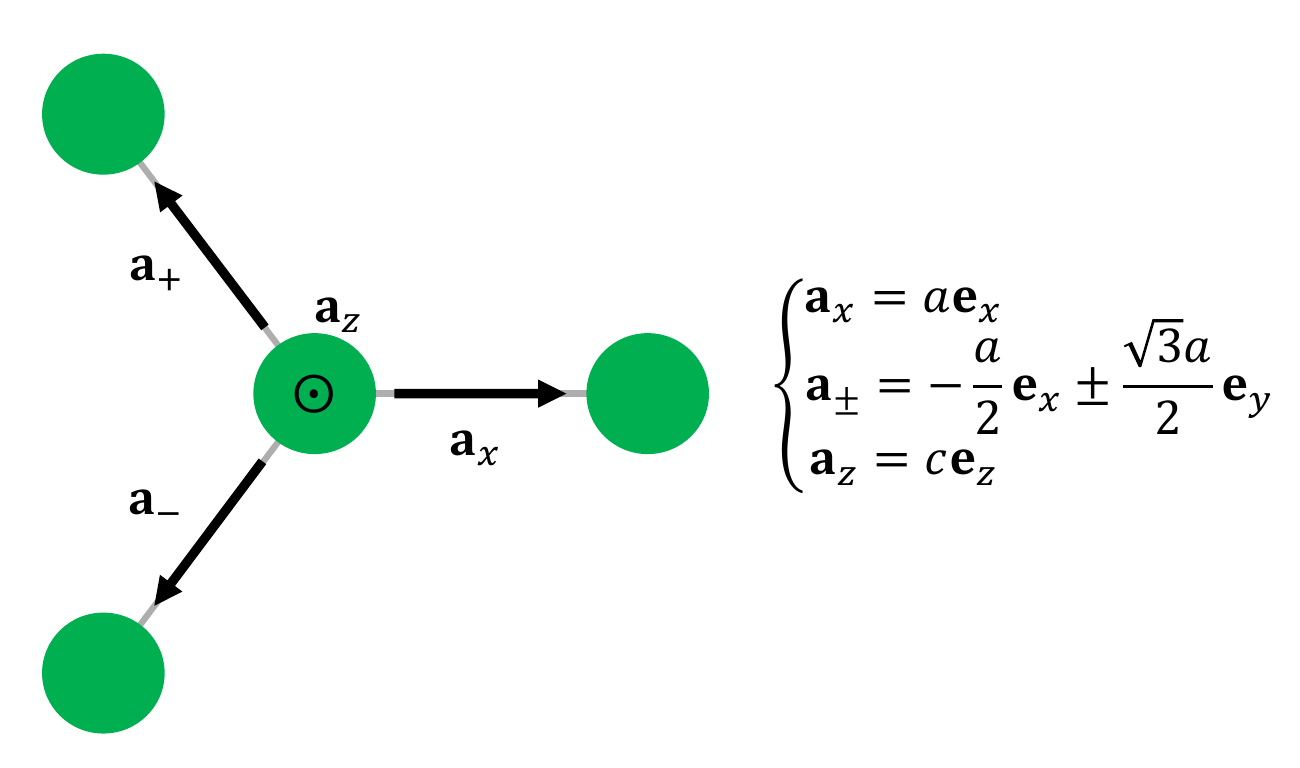} % Adjust width as needed
		}
		\caption{Schematic of the simple unit cell and its vectors in the $D_3$ materials.}
	\end{figure}
	
%	\clearpage
	We now apply the projection operator to the unit cell vectors and obtain the projected components for each irreducible representation.\\
	\textbf{$A_1$ irrep.}
	\begin{align*}
		\phi_{A_1} &\propto 1 \cdot \mathbf{a}_x + 1 \cdot \mathbf{a}_x + 1 \cdot \mathbf{a}_- + 1 \cdot \mathbf{a}_+ + 1 \cdot \mathbf{a}_+ + 1 \cdot \mathbf{a}_- = 0 \\
		\phi_{A_1} &\propto 1 \cdot \mathbf{a}_z - 1 \cdot \mathbf{a}_z - 1 \cdot \mathbf{a}_z - 1 \cdot \mathbf{a}_z + 1 \cdot \mathbf{a}_z + 1 \cdot \mathbf{a}_z = 0
	\end{align*}
	
	\noindent\textbf{$A_2$ irrep.}
	\begin{align*}
		\phi_{A_2} &\propto 1 \cdot \mathbf{a}_x + (-1) \cdot \mathbf{a}_x + (-1) \cdot \mathbf{a}_- + (-1) \cdot \mathbf{a}_+ + 1 \cdot \mathbf{a}_+ + 1 \cdot \mathbf{a}_- = 0 \\
		\phi_{A_2} &\propto 1 \cdot \mathbf{a}_z - (-1) \cdot \mathbf{a}_z - (-1) \cdot \mathbf{a}_z - (-1) \cdot \mathbf{a}_z + 1 \cdot \mathbf{a}_z + 1 \cdot \mathbf{a}_z \propto \mathbf{e}_z
	\end{align*}
	
	\noindent\textbf{$E$ irrep.}
	\begin{align*}
		\phi_{E(1)} &\propto 1 \cdot \mathbf{a}_x + 1 \cdot \mathbf{a}_x + \left(-\frac{1}{2}\right) \cdot \mathbf{a}_- + \left(-\frac{1}{2}\right) \cdot \mathbf{a}_+ + \left(-\frac{1}{2}\right) \cdot \mathbf{a}_+ + \left(-\frac{1}{2}\right) \cdot \mathbf{a}_- \propto \mathbf{e}_x \\
		\phi_{E(2)} &\propto 0 \cdot \mathbf{a}_x + 0 \cdot \mathbf{a}_x + \left(-\frac{\sqrt{3}}{2}\right) \cdot \mathbf{a}_- + \left(\frac{\sqrt{3}}{2}\right) \cdot \mathbf{a}_+ + \left(\frac{\sqrt{3}}{2}\right) \cdot \mathbf{a}_+ + \left(-\frac{\sqrt{3}}{2}\right) \cdot \mathbf{a}_- \propto \mathbf{e}_y,
	\end{align*}
	These results indicate that $\phi_{A_2}$ contributes to the $z$ component ($\mathbf{e}_z$), $\phi_{{E}(1)}$ to the $x$ component ($\mathbf{e}_x$), and $\phi_{{E}(2)}$ to the $y$ component ($\mathbf{e}_y$).

    We next apply the same projection procedure to the angular momentum with periodicity in the Brillouin zone. Focusing only on the periodic part, we express the angular momentum as phase factors,
	\begin{align}
		|\mathbf{L}_j(\mathbf{k})| \sim e^{i\mathbf{k} \cdot \mathbf{a}_x}, e^{i\mathbf{k} \cdot \mathbf{a}_z}.
	\end{align}
	Using Fig.~S7, Table~S3 can be constructed from the relations: $p_x = e^{i\mathbf{k} \cdot \mathbf{a}_x}$, $p_{\pm} = e^{i\mathbf{k} \cdot \mathbf{a}_{\pm}}$, and $p_z = e^{i\mathbf{k} \cdot \mathbf{a}_z}$.
	\begin{table}[h]
		\centering
		\renewcommand{\arraystretch}{1.5}
		\begin{tabular}{c c c c c c c}
			\toprule
			irrep. & $1$ & $C_2$ & $C_2$ & $C_2$ & $C_3$ & $C_3^{-1}$ \\
			\midrule
			$A_1$ & 1 & 1 & 1 & 1 & 1 & 1 \\
			$A_2$ & 1 & $-1$ & $-1$ & $-1$ & 1 & 1 \\
			\midrule
			$E$ & 
			$\begin{pmatrix} 1 & 0 \\ 0 & 1 \end{pmatrix}$ & 
			$\begin{pmatrix} 1 & 0 \\ 0 & -1 \end{pmatrix}$ & 
			$\begin{pmatrix} -\frac{1}{2} & -\frac{\sqrt{3}}{2} \\ -\frac{\sqrt{3}}{2} & \frac{1}{2} \end{pmatrix}$ & 
			$\begin{pmatrix} -\frac{1}{2} & \frac{\sqrt{3}}{2} \\ \frac{\sqrt{3}}{2} & \frac{1}{2} \end{pmatrix}$ & 
			$\begin{pmatrix} -\frac{1}{2} & -\frac{\sqrt{3}}{2} \\ -\frac{\sqrt{3}}{2} & -\frac{1}{2} \end{pmatrix}$ & 
			$\begin{pmatrix} -\frac{1}{2} & \frac{\sqrt{3}}{2} \\ \frac{\sqrt{3}}{2} & -\frac{1}{2} \end{pmatrix}$ \\
			\midrule
			$\chi_E$ & 2 & 0 & 0 & 0 & $-1$ & $-1$ \\
			\bottomrule
			\toprule
			$\mathcal{G}[p_x]$ & $p_x$ & $p_x$ & $p_-$ & $p_+$ & $p_+$ & $p_-$ \\
			$\mathcal{G}[p_z]$ & $p_z$ & $-p_z$ & $-p_z$ & $-p_z$ & $p_z$ & $p_z$ \\
			\bottomrule
		\end{tabular}
		\caption{Irreducible representations of $D_3$ and symmetry operations acting on angular momentum (phase factors).}
	\end{table}
	
	The phase factors for each irreducible representation can be obtained as follows.\\
	\textbf{$A_1$ irrep.}
	\[
	\phi_{A_1} \propto 1 \cdot p_x + 1 \cdot p_- + 1 \cdot p_+ + 1 \cdot p_+ + 1 \cdot p_- \propto p_x + p_+ + p_-
	\]
	\[
	= e^{ik_x a} + 2 e^{-ik_x a/2} \cos\left(\frac{\sqrt{3}}{2} k_y a \right)
	\]
	\[
	\phi_{A_1} \propto 1 \cdot p_z + 1 \cdot p_z^* + 1 \cdot p_z^* + 1 \cdot p_z^* + 1 \cdot p_z + 1 \cdot p_z \propto p_z + p_z^* = 2 \cos k_z c
	\]
	
	\noindent\textbf{$A_2$ irrep.}
	\[
	\phi_{A_2} \propto 1 \cdot p_x + (-1) \cdot p_x + (-1) \cdot p_- + (-1) \cdot p_+ + 1 \cdot p_+ + 1 \cdot p_- = 0
	\]
	\[
	\phi_{A_2} \propto 1 \cdot p_z + (-1) \cdot p_z^* + (-1) \cdot p_z^* + (-1) \cdot p_z^* + 1 \cdot p_z + 1 \cdot p_z \propto p_z - p_z^*= 2i \sin k_z c
	\]
	
	\noindent\textbf{$E$ irrep.}
	\[
	\phi_{E_{(1)}} = 1 \cdot p_x + 1 \cdot p_x + \left(-\frac{1}{2}\right) \cdot p_- + \left(-\frac{1}{2}\right) \cdot p_+ + \left(-\frac{1}{2}\right) \cdot p_+ + \left(-\frac{1}{2}\right) \cdot p_- 
	\]
	\[
	\propto p_x - (p_+ + p_-)
	= e^{ik_x a} - 2e^{-ik_x a/2} \cos\left(\frac{\sqrt{3}}{2} k_y a \right)
	\]
	\[
	\phi_{E_{(2)}} \propto 0 \cdot p_x + 0 \cdot p_x + \left(-\frac{\sqrt{3}}{2}\right) \cdot p_- + \left(\frac{\sqrt{3}}{2}\right) \cdot p_+ + \left(\frac{\sqrt{3}}{2}\right) \cdot p_+ + \left(-\frac{\sqrt{3}}{2}\right) \cdot p_-
	\]
	\[
	\propto p_+ - p_-
	= 2i e^{-ik_x a/2} \sin\left(\frac{\sqrt{3}}{2} k_y a\right)
	\]
	Therefore, each component of the structure factor can be constructed from the phase factors of the $A_2$ and $E$ irreducible representations.
	\[
	{A_2\ \text{irrep.}} \quad F_1^z
	\]
	\[
	{E\ \text{irrep.}} \quad (F_1^x, F_1^y)
	\]
	After expressing the exponential terms again in trigonometric functions, the structure factors are then obtained as given in Eq.~(S4). Similarly, the structure factors for $O_h$ and $T_d$ can be derived as shown in Eq.~(S5). The coefficients of the structure factors are determined by normalization over the entire Brillouin zone.
	
%\newpage
\section{Alternative validation and computational details}

To cross-validate the proposed measures of phonon chirality, we performed calculations using an alternative first-principles approach based on the finite-displacement method, as implemented in the \textsc{phonopy} package~\cite{Togo2015} in combination with the \textsc{VASP} code~\cite{Kresse1996}.

\subsection{Computational setup}

All calculations were carried out within density functional theory using the projector augmented-wave (PAW) method as implemented in \textsc{VASP}. The exchange--correlation functional was treated within the generalized gradient approximation (GGA) in the Perdew--Burke--Ernzerhof (PBE) form. Representative computational parameters are summarized in Table~S4. Atomic displacements of $0.01~\text{\AA}$ were employed in the finite-displacement calculations.

Phonon properties were computed using \textsc{phonopy}, and the phonon angular momentum and dynamical chirality were evaluated from the obtained eigenfrequencies and eigendisplacements following the definitions in the main text. The bulk dynamical chirality $G_0$ and $G_u$ were computed by summing over phonon modes on a uniform $q$-point mesh of $21\times21\times21$ at $T=300~\mathrm{K}$.

\subsection{Consistency with DFPT results}

The calculations using the alternative approach reproduce the key qualitative features reported in the main text. In particular,
(i) the momentum-resolved dynamical chirality changes sign between enantiomers across the Brillouin zone,
(ii) centrosymmetric crystals exhibit vanishing chirality at all wave vectors, and
(iii) noncentrosymmetric achiral crystals show finite local chirality that cancels in the Brillouin-zone sum, resulting in vanishing bulk dynamical chirality.

These results confirm that the symmetry-based characterization of phonon chirality is robust across different computational approaches.

\subsection{Quantitative differences}

While the qualitative behavior is consistent, quantitative differences in the values of $G_0$ and $G_u$ are observed between the finite-displacement and density-functional perturbation theory (DFPT) calculations used in the main text. Representative comparisons are summarized in Table~S5.

These differences can arise from several sources, including the choice of computational method (finite displacement vs DFPT), the use of different pseudopotentials, convergence with respect to supercell size and $q$-point sampling, and small variations in relaxed atomic structures. In particular, the projection of phonon angular momentum onto symmetry-adapted structure factors can be sensitive to subtle differences in atomic positions.

Overall, these calculations using an alternative approach support the generality of the proposed framework while indicating that quantitative comparisons of $G_0$ and $G_u$ should be made within a consistent computational setup.

\begin{table}[t]
\caption{Representative computational parameters used in the finite-displacement calculations.}
\begin{tabular}{lcccc}
\toprule
Material & ENCUT (eV) & Supercell & $k$-mesh & NAC \\
\midrule
R-SiO$_2$ & 600 & $3\times3\times2$ & $\Gamma$ & Yes \\
Si        & 520 & $4\times4\times4$ & $\Gamma$ & Yes \\
GaAs      & 500 & $4\times4\times4$ & $\Gamma$ & Yes \\
\bottomrule
\end{tabular}
\label{tab:params_VASP}
\end{table}

\begin{table}[t]
\caption{Comparison of bulk dynamical chirality obtained from DFPT and finite-displacement (FD) calculations.}
\begin{tabular}{lcccc}
\toprule
Material & $G_0$ (DFPT) & $G_0$ (FD) & $G_u$ (DFPT) & $G_u$ (FD) \\
\midrule
R-SiO$_2$ & 0.42 & 0.25 & $-0.11$ & $-0.04$ \\
Si        & 0.00 & 0.00 & 0.00 & 0.00 \\
GaAs      & 0.00 & 0.00 & 0.00 & 0.00 \\
\bottomrule
\end{tabular}
\label{tab:comparison}
\end{table}

\end{document}
